# Supplementary material for: Counterfactual Editing for Search Result Explanation
Source: arXiv:2301.10389 source file (2024-06-28)
Supplement: Supplementary file 1 [file appendix.tex]

\section{Qualitative Studies}
\label{appendix:qualitative}
Here we showcase a few examples of the success and failure of the proposed \method. All these examples are from MS MARCO dataset dev subset.

\begin{minipage}{0.9\columnwidth}
\begin{center}
\vspace{5pt}
\begin{tcolorbox}[width=\columnwidth]
\textbf{Initial query}: what is process control equipment \\
\textbf{Top-1 document}: what is process control? process control is an algorithm that is used in the during the manufacturing process in the industries for the active changing process based on the output of process monitoring. \\
\textbf{Counterfactual document}: process equipment is equipment used in chemical and materials processing, in facilities like refineries, chemical plants, and wastewater treatment plants. this equipment is usually designed with a specific process or family of processes in mind and can be customized for a particular facility in some cases. \\
\textbf{Counterfactual query}: what is process \textbf{\st{control}} \textbf{\textcolor{blue}{[PAD]}} equipment
\end{tcolorbox}
\vspace{5pt}
\end{center}

In the above example, we can see \method captures the topic difference between top ranked document and 2nd ranked document, and it provides a reasonable explanation for the pairwise relevance relation, i.e. to remove the keyword \textbf{control}.

\end{minipage}

\begin{minipage}{0.9\columnwidth}
\begin{center}
\vspace{5pt}
\begin{tcolorbox}[width=\linewidth]

\textbf{Initial query}: cost of attendance eastern illinois university \\
\textbf{Top-1 document}: eastern illinois university has roughly 8,000 students. admission is selective. tuition is approximately \$8,550 per year for residents of illinois and other bordering states, while it is \$10,680 for non-residents. additional fees amount to \$2,762.32. the university estimates its average cost-of-attendance to be approximately \$24,640 per academic year. tuition is expected to increase in the 2016 - 2017 academic year. \\
\textbf{Counterfactual document}: the cost of attending northern illinois university for in-state students without financial aid is \$14,295. the cost for out-of-state students without financial aid is \$23,761. \\
\textbf{Counterfactual query}: cost of attendance \textbf{\st{eastern}} \textbf{\textcolor{blue}{northern}} illinois university

\end{tcolorbox}
\vspace{5pt}
\end{center}

In the above example, we can see the 3rd ranked document is about northern illinois university, and \method successfully captures the difference and suggests a reasonable and informative counterfactual query.

\end{minipage}

\begin{minipage}{0.9\columnwidth}
\begin{center}
\begin{tcolorbox}[width=\linewidth]
\textbf{Initial query}: how long is a typical car loan? \\
\textbf{Top-1 document}: in general, car loans are structured to offer 12 - month increments and last somewhere between two and eight years. that means you'll find available loans of 24 months, 36 months, 48 months, 60 months, 72 months and 84 months. the average new car loan is around 65 months, or more than five - and - a - half years, while the average used car loan is shorter. long - term drawbacks. when you're signing the paperwork at the dealer, you'll be tempted to go for a longer term \\
\textbf{Counterfactual document}: if you're in the market for a new car, the length of the average auto loan may surprise you. loans for many years were typically around five years, or 60 months. buyers now seek varying loan lengths and terms, depending on the vehicle and the state of the economy at the time of purchase. \\
\textbf{Counterfactual query}: how long is a typical \textbf{\st{car}} \textbf{\textcolor{blue}{automobile}} loan?
\end{tcolorbox}
\end{center}
\vspace{5pt}

In the above example we can see although \method captures the keyword \textbf{auto} in the counterfactual document, it fails to predict an informingly different query. 
This is partially due to the similarity between the top-1 ranked document and the lower ranked counterfactual document. 
This suggests that when the counterfactual document also addresses the information need of the initial query, \method may fail to produce a sufficiently different counterfactual query as explanation.
\end{minipage}
